# Supplementary material for: Effects of hole self-trapping by polarons on transport and negative bias illumination stress in amorphous-IGZO
Source: arXiv:1709.03728 ancillary file (2017-09-12)
Supplement: Supplementary file 1 [file sup.pdf]

# Influence of hole self-trapping on NBIS in amorphous IGZO - Supplementary material

A. de Jamblinne de Meux[1,2], G. Pourtois[2,3],
J. Genoe[1,2] and P. Heremans[1,2]

July 7, 2017

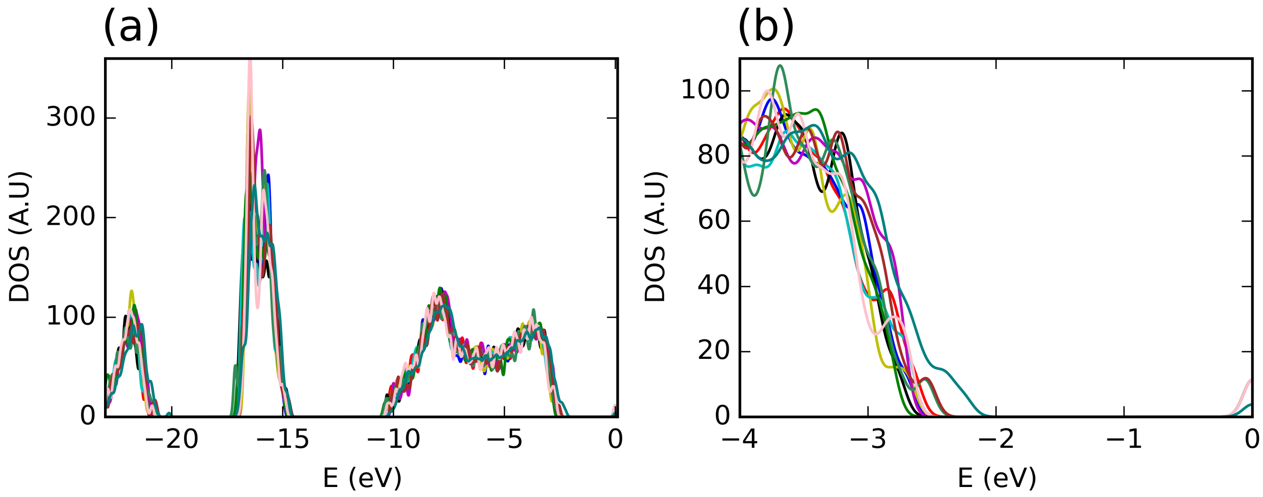


Figure 1: Density of states of the 11 models of a-IGZO. The zero of the energy axis is set at the conduction band. Panel (a) provides the complete energy range while panel (b) zooms on the gap region.

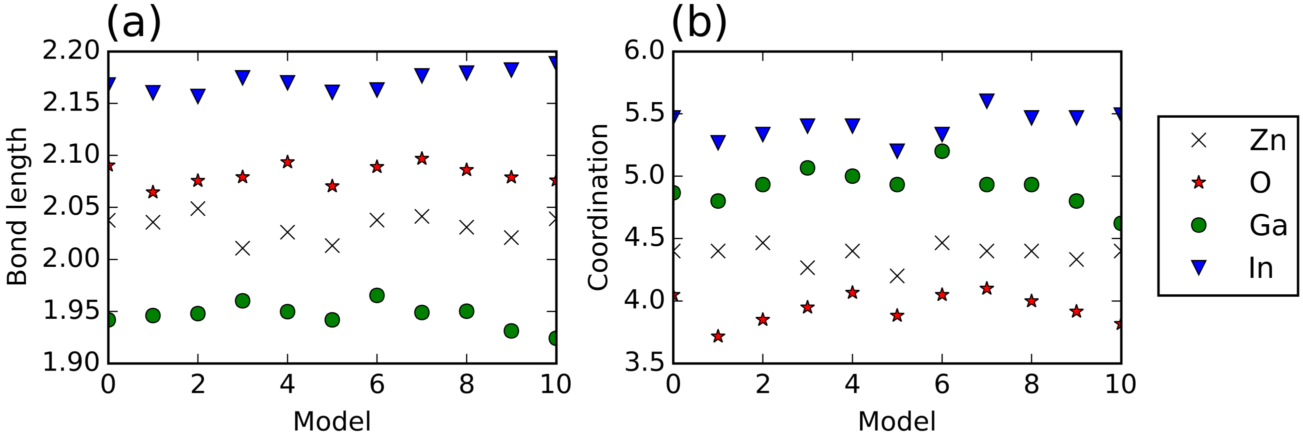


Figure 2: Structural parameters of the different models. (a) Mean bond lengths and (b) mean coordinations numbers. The 315 atoms model is labeled 10.

| Model | Total Energy (eV/atom) |
|---|---|
| 0 | 0.1205 |
| 1 | 0.1285 |
| 2 | 0.1112 |
| 3 | 0.1154 |
| 4 | 0.1118 |
| 5 | 0.1185 |
| 6 | 0.1272 |
| 7 | 0.1174 |
| 8 | 0.1282 |
| 9 | 0.1284 |
| 10 | 0.1656 |

Table 1: Formation energies of the different amorphous structures using crystalline IGZO as reference. As expected, all the structures are meta-stable in regards to crystalline IGZO.
